# Supplementary material for: Work Practices and Perceptions from Women Core Developers in OSS Communities
Source: arXiv:2007.13891 source file (2020-07-27)
Supplement: Supplementary file 1 [file 8_appendix.tex]

\appendix

\begin{table*}[htb!]
    \centering
    \caption{Suggestion to increase women's participation in the open source Communities todo}
    \label{tab:suggestion}
    \begin{tabular}{|p{0.45cm}|p{16.5cm}|} 
    \hline
ID & Key developers suggestion   
\\ \hline
R1 &  Communities can encourage woman as a co-mentor if they are not mentors, this will help women contributors to be more comfortable to interact with them.  
\\ \hline
R2 & Motivate them from a young age.  
\\ \hline
R3 & Communication, awareness, women in tech to organize and participate in events. 
\\ \hline
R4 & Encouragement.
\\ \hline
R5 & Have more examples, namely role models in the open source community. 
\\ \hline
R6 & Promote a general discussion/research on why women's participation is so low. There can be more than one reason. Usual "rude" behavior may be one of them, but not the only one. And it is important to consider that women's participation in Computing is currently also low, and has been higher. 
\\ \hline
R7 & Start women coding challenges with mentorship programs. 
\\ \hline
R8 & Organizing more webinars and meetups. 
\\ \hline
R9 & Having more women promoting open source projects and work, through blogs, forums, public speaking, helping to demystify the world of open source. Have women maintainers, real examples others can see. 
\\ \hline
R10 & Educate men to behave. 
\\ \hline
R11 & Have mentors encourage more women to do it. I got involved as someone more senior suggested I should.  
\\ \hline
R12 & Popularizing OSS contributions in companies; there is not enough visibility for most OSS projects and how to contribute to them. 
\\ \hline
R13 & More mentorship programs. 
\\ \hline
R14 & Increase gender diversity in programming in general. 
\\ \hline
R15 & Local meetups. 
\\ \hline
R16 & Have a proportion of project for women. 
\\ \hline
R17 & Publicize things like Outreachy.
\\ \hline
R18 & Let people know that thy can contribute regardless of gender, political views or religion, country of origin, etc. 
\\ \hline
R19 & Women are participating, but their performance does not get the same positive reaction as men's. To get more women to participate, that reception should change. 
\\ \hline
R20 & Organize programs and events specially targeted to women. 
\\ \hline
R21 & Inform women’s group more, through universities and communities.
\\ \hline
R22 & Outreach to woman in various communities and cultures. 
\\ \hline
R23 & I feel that the solution is to build confidence. Every approach towards increasing participation of women has a side that increases confidence and another that decreases it. The one that I completely support is building a peer group among girls interested in it. It is not so common to find many girls in technical teams and also, it is not considered cool to be a techie girl. (There's a lot of peer pressure when you're not with people of common interests. That's what I felt until I actually told the truth and found my girly tech community). I'm a very introverted person. I rarely even communicate with anyone on those online chat platforms (even though we have a girls group over there as well). So, having people around me with whom I can share everything that I do every day without having a fear of being judged as a freak, has been pretty helpful and encouraging.  
\\ \hline
R24 & More programs like Outreach.
\\ \hline
R25 & Conferences for women in tech just to promote OSS contribution right from their early career. Familiarizing them with opportunities like GSoC, RGSoC, Outreachy etc.  
\\ \hline
R26 &  I started participating because I had the chance to get a little stipend for my open source work. After the initial incentive to top up by student budget I realized how much fun it is and stuck to it ever since. I think I would not have started without that, because it always seemed more like a guys hangout and usually you have to be of a very outgoing personality to make first friends in a guys only club. 
\\ \hline
R27 & Meetups and community bonding. 
\\ \hline
R28 & Any sort of compensation. 
\\ \hline
R29 & Inform more about opportunities in the open source world. 
\\ \hline
R30 & Encourage more women to get into coding. 
\\ \hline
R31 & More awareness and tech support groups. \\ \hline
    \end{tabular}
    \end{table*}

\begin{table*}[htb!]
    \centering
     \caption{Suggestion to create a more inclusive environment for women in open source communities}
    \begin{tabular}{|p{0.45cm}|p{16.5cm}|}
    \hline
        ID & Opinion \\ \hline
      R1  & I think women are doing great in OSS, just a little more recognition and appreciating will motivate them and encourage new women to step into OSS. \\ \hline
      R2 & Stop treating women developers as ``women developers'' and start treating them as developers. \\ \hline
      R3 & It should be inclusive for everyone, regardless of gender or other characteristics. Talk about it, raise awareness, psychology and self development has a lot to teach us. \\ \hline
      R4 & Programs like Outreachy help a lot.
      \\ \hline
      R5 & Have more women members and mentors in organizations.
      \\ \hline
      R6 & OSS Communities should be inclusive not only for women, but for all (men, women, LGBT..., disabled, etc).
      \\ \hline
      R7 & Less men.
      \\ \hline
      R8 & Mentorship program at school level.
      \\ \hline
      R9 & Allowing gender diversity.
      \\ \hline
      R10 & Have a clear Code of Conducts and a way to report abuses to Community Managers. Avoid gender pronouns (e.g.: using "guys" is very common, and this gives an idea that it is assumed that contributors are mostly men), so moderating language would help.
      \\ \hline
      R11 & Educate men to behave properly.
      \\ \hline
      R12 & Have more diverse involvement and then more diverse people will want to join in. But you need that to start somewhere, it is a slow change but it is going in the right direction.
      \\ \hline
      R13 & Establishing good communication.
      \\ \hline
      R14 & Promote more women to senior role, prevent incidents of man-explaining.
      \\ \hline
      R15 & Establish a code of conduct for OSS projects where feedback is encouraged to be empathetic, encouraging, and supportive of all contributions.
      \\ \hline
      R16 & Inspite of organizing exclusive women events, organize events that are equal for everyone.
      \\ \hline
      R17 & Incentive woman participation at all levels, if the OSS reference are most men this is a problem. Promote women contributions in the community.
      \\ \hline
      R18 & Get more of them to participate.
      \\ \hline
      R19 & If the family does not have a positive environment for woman, then start working with the family to change their way of thinking (very difficult when religion is part of the cause). Otherwise, let know the woman not to fear when contributing, she will be treated just like anyone else: good contribution then its accepted regardless of gender, political views or religion, country of origin, etc., bad contributions are not accepted regardless of gender, political views or religion, country of origin, etc.
      \\ \hline
      R20 & In the R community there are R-Ladies events - held by and for women. Girl only or (predominantly) events in general, could create an environment that suggests that girls and women are actually wanted to be included in the community. Going for gender balance and diversity in hackathons or other OSS events helps. It also helps to celebrate achievements and invite more women to keynote events.
      \\ \hline
      R21 & I think OSS communities are quite inclusive but lack a minimum percentage of women contributors.
      \\ \hline
      R22 & We need to support women in educational programs environments more.
      \\ \hline
      R23 & Placing more women in leadership positions will encourage a more open and inclusive environment that would hopefully encourage more diverse participation.
      \\ \hline
      R24 & A good code of conduct and a good admin is all you need.
        \\ \hline
        R25 & By motivating them to work on more issues and features.
         \\ \hline
         R26 & Some projects reserved for women.
          \\ \hline
         R27 & Don't focus so much on 'important' very basic packages (e.g. Numpy, Scipy) but more on the smaller ones, e.g. important only in a couple specific domains (like PySAL or geopandas). You are much more likely to encourage women participation here. You will not limit yourself to attract women that have a classical computer science background, but e.g. women in earth system sciences, who are also technically inclined but have not come into direct contact with e.g. software development. You open up the pool of women to reach out to and you eliminate the danger of the 'I do not have enough skills for that' thinking.
          \\ \hline
          R28 & Meetups.
            \\ \hline
          R29 & Honestly, I wish I knew more about how to better support inclusivity.
             \\ \hline
             R30 & Increase projects such as outreachy.
              \\ \hline
              R31 & If OSS communities host overnight hackathons, make sure to provide more or less comfortable place to sleep.
              \\ \hline
              R32 & Have closed forums for women to talk about their experiences.
                \\ \hline
      \end{tabular}
      \label{tab:my_label14}
\end{table*}
